# Supplementary material for: Hidden Silicon-Vacancy Centers in Diamond
Source: arXiv:2006.02323 ancillary file (2021-05-05)
Supplement: Supplementary file 1 [file SiVcompare_SM8.pdf]

# Supplemental Material:
# Hidden Silicon-Vacancy Centers in Diamond

Christopher L. Smallwood,[1,2] Ronald Ulbricht,[3] Matthew W. Day,[1] Tim Schröder,[4,5] Kelsey M. Bates,[1] Travis M. Autry,[6,7,*] Geoffrey Diederich,[8,†] Edward Bielejec,[9] Mark E. Siemens,[8] and Steven T. Cundiff[1,‡]

[1]*Department of Physics, University of Michigan, Ann Arbor, MI 48109, USA*

[2]*Department of Physics and Astronomy, San José State University, San Jose, CA 95192, USA*

[3]*Max Planck Institute for Polymer Research, Ackermannweg 10, 55128 Mainz, Germany*

[4]*Department of Electrical Engineering and Computer Science, Massachusetts Institute of Technology, Cambridge, MA 02138, USA*

[5]*Department of Physics, Humboldt-Universität zu Berlin, Newtonstraße 15, 12489 Berlin, Germany*

[6]*JILA, University of Colorado & National Institute of Standards and Technology, Boulder, CO 80309, USA*

[7]*Department of Physics, University of Colorado, Boulder, CO 80309, USA*

[8]*Department of Physics and Astronomy, University of Denver, Denver, CO 80208, USA*

[9]*Sandia National Laboratories, Albuquerque, NM 87185, USA*

(Dated: March 22, 2021)

## SAMPLE

The silicon-vacancy sample measured was a chemical-vapor deposition grown, (110)-oriented sample of single-crystal diamond from Element Six (standard type-IIa electronic-grade sample, about 5 ppb nitrogen concentration) that was approximately 2 mm wide, 2 mm long, and 0.3 mm thick. The diamond sample was mechanically polished and chemically etched to produce a smooth surface. A high-density ensemble of $SiV^-$ centers was created by implanting silicon-29 ions with an ion beam at depths between 0.5 and 2.4 $\mu$m using a range of beam energies from 0.8 to 8 MeV in four different 800 $\times$ 800 $\mu$m squares. The sample was then annealed at 1000–1050° C and tri-acid cleaned. An anti-reflective coating was applied to reduce coherent scatter and reject reflections from the face of the sample. Figure S1 shows a picture of the sample with the relevant electric field orientation and a cartoon of the sample orientation. The excitation electric field was polarized horizontally with respect to the sample face. Figure S2 depicts the implantation parameters used for one square of ion implantation. The sample was measured in a closed-circuit cryostat, in cryogenic conditions under vacuum.

It is argued in the main text that the most likely generator of the hidden $SiV^-$ center distribution is strain. As displayed in Fig. S2 the sample measured in this study consists of an unusually high concentration of implanted silicon ions—about $8 \times 10^{18}$ atoms/cm$^3$ within the 500–2250 nm implantation depth. A back-of-the envelope calculation indicates that this corresponds to a relatively small average strain (on the order of $2 \times 10^{-5}$). However,

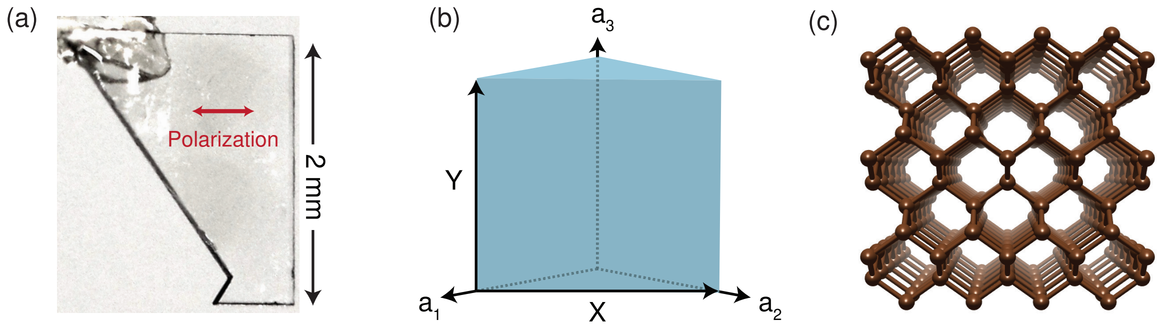


FIG. S1. Details of the (110) sample and electric field configuration. **(a)** Sample photograph. **(b)** Orientation of the $a_1$, $a_2$, and $a_3$ basis vectors relative to the sample surface. **(c)** Ball-and-stick model of the diamond lattice as viewed looking down at the sample surface.

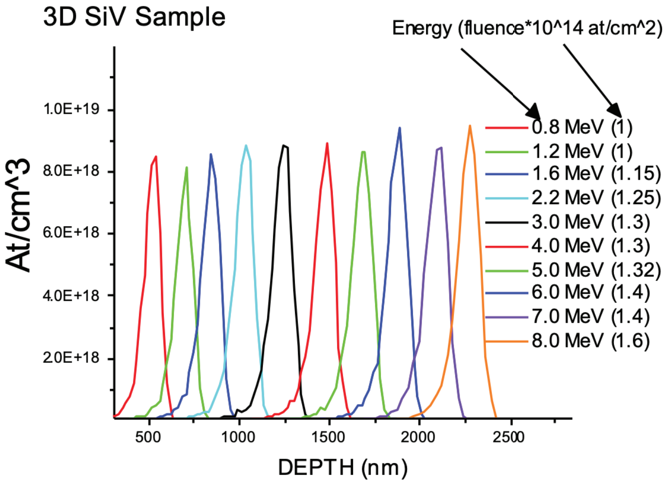


FIG. S2. Parameters used to implant $^{29}$Si atoms into the diamond lattice. The implantation depth was varied by changing the beam energy and the fluence was held between $1 \times 10^{14}$ and $2 \times 10^{14}$ atoms/cm$^2$.

the implantation process likely distributes this strain throughout the crystal in a highly inhomogeneous fashion, and there is evidence that SiV$^-$ centers prefer to form at high-strain locations in diamond like grain boundaries and morphological defects [1]. The inhomogeneity would in turn produce significantly larger strain values on a microscopic level than would be conceivable to generate using other methods such as the cantilever method demonstrated by Meesala, et al. [2].

An alternate explanation for modified color-center spectral properties is electrostatic surface effects. As displayed in Fig. S2, however, the bulk of the sample's SiV$^-$ centers were implanted at depths ranging from 500–2250 nm whereas diamond surface effects are expected to taper off at depths exceeding 50 nm [3, 4]. A depth-dependent yield could in principle lead to depth-dependent spectra. It was shown for SiV$^-$ centers specifically, however, that for depths between 15 nm and 68 nm the yield stays constant [5]. A constant yield is also expected for depths greater than 68 nm. The depth dependence consequently seems unlikely to exert a measurable impact on SiV$^-$ center dynamics.

## MDCS MEASUREMENTS

Figures S3 and S4 show detailed schematics for the multidimensional coherent spectroscopy (MDCS) experiments described in the main text, which are photoluminescence-detected MDCS (Fig. S3) and heterodyne-detected MDCS (Fig. S4). The measurements in both cases employ a collinear excitation pulse geometry that is a variant of experimental setups described by Tekavec, et al. [6], Nardin, et al. [7], and Martin and Cundiff [8]. The experiment works as follows: pulses are generated by a titanium-sapphire (Ti:Sapph) oscillator and sent into two Mach-Zehnder interferometers nested within a third (constituting a four-armed interferometer). We label the arms $A$, $B$, $C$, and $D$ as shown in figures S3 and S4. Time delays $\tau$ and $t$ are controlled by delay stages along arms $A$ and $D$ of the interferometer. The time delay $T$ is controlled by a delay stage between the two smaller interferometers that serves to delay pulses along arms $C$ and $D$ relative to pulses along arms $A$ and $B$. The main text reports one-quantum rephasing spectra, establishing the correspondences

$$\begin{aligned} &\text{Pulse } A \leftrightarrow \text{Pulse 1} \quad &&\text{(First-order interaction)}\\ &\text{Pulse } B \leftrightarrow \text{Pulse 2} \quad &&\text{(Second-order interaction)}\\ &\text{Pulse } C \leftrightarrow \text{Pulse 3} \quad &&\text{(Third-order interaction)}\\ &\text{Pulse } D \leftrightarrow \text{Pulse 4} \quad &&\text{(Fourth-order interaction or local oscillator).} \end{aligned}$$

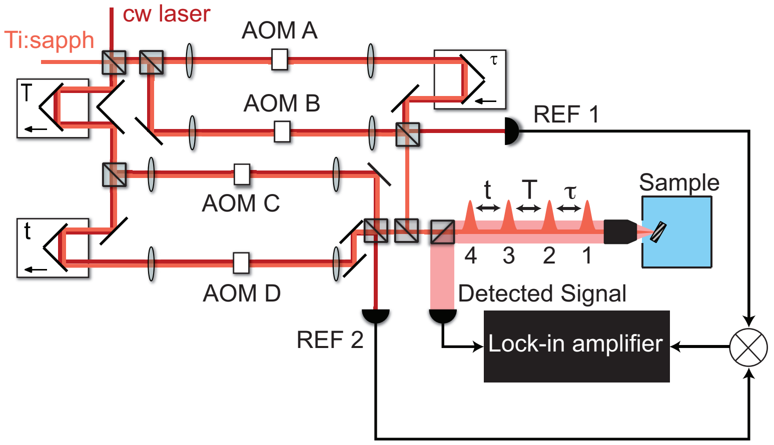


FIG. S3. A depiction of the photoluminescence detected MDCS experiment. All four pulses are routed onto the sample.

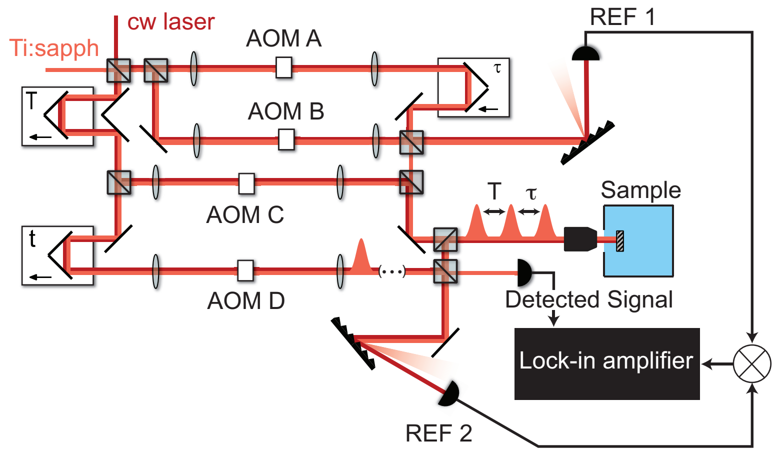


FIG. S4. A depiction of the heterodyne-detected MDCS experiment. Three of four pulses are routed onto the sample, and the third-order coherent emission is collected and interfered with pulse $D$, which is routed directly to the detector.

To isolate the MDCS signal, the pulses traveling through each of these four arms are frequency-tagged by using acousto-optic modulators (AOMs) driven by radio-frequency offsets $\nu_A = 81.135$ MHz, $\nu_B = 81.000$ MHz, $\nu_C = 79.085$ MHz, and $\nu_D = 79.000$ MHz, resulting in a nonlinear beatnote in the detected optical signal at the frequency $\nu_{sig} = -\nu_A + \nu_B + \nu_C - \nu_D = 50$ kHz, which is filtered and detected using a lock-in amplifier. Pulses are directed toward the sample and collected from the sample using a microscope objective of NA $= 0.4$, resulting in a beam spot roughly 2.5 $\mu$m in diameter. In the case of the PL-detected measurements (Fig. S3), all four of the beams are directed onto the sample, and the signal is observed as an intensity modulation in the emitted PL. To isolate the signal from coherent emission, the sample was rotated relative to the excitation beams by an angle of 30 degrees. In the case of the heterodyne-detected measurements (Fig. S4), the beatnote is created by mixing Pulse $D$ with the coherent emission signal emitted in reflection by the interaction of the sample with pulses $A$–$C$. The sample was oriented directly normal to the excitation beams in this case. In both cases, the measurements' multidimensional character comes from recording the amplitude and phase of the lock-in amplifier signal as a function of time delays $\tau$ and $t$, and then performing a two-dimensional numerical Fourier transform to bring these spectra into the frequency domain.

To ensure the relative phase stability of our measurements, a continuous wave (CW) laser is directed along the same interferometer arms as the pulsed laser, for the purpose of detect-

ing and electronically subtracting the unavoidable interferometer path length fluctuations [7]. Upon being collected, the two signals are mixed using a field-programmable gate array (FPGA) to produce a difference frequency, which is in turn fed into the lock-in amplifier's external reference input. In the case of PL detection, the CW laser is spatially and spectrally offset from the Ti:Sapph in all four interferometer arms, enabling easy separation between the two laser signatures at photodetectors detectors REF 1 and REF 2. In the case of heterodyne detection, the $A/B$ beatnote is collected at REF 1 as before, but the CW laser is arranged collinearly to beam $C$ so that it can be sent onto the sample and interfered with the CW laser collinear with beam $D$ at REF 2 [8]. Thus, the $C/D$ beatnote of the CW laser is separated from the beatnotes induced by the Ti:sapph using spectral separation only, and not spatial separation.

## PHOTOLUMINESCENCE

The conventional photoluminescence measurement of the $\mathrm{SiV}^-$ center sample depicted by the blue trace in Fig. 2(a) of the main text was collected with linearly polarized pulsed light from the Ti:sapphire oscillator (≈7.5 nm bandwidth or 100-fs pulse duration), with scattered light suppression achieved through cross-polarized signal detection. The PL in this measurement was directed through a single-mode, polarization-maintaining fiber onto a grating spectrometer with a spectral resolution of 24 GHz, full-width at half-maximum (FWHM). We determined the resolution experimentally using an argon line from a spectrometer calibration lamp.

## BACKGROUND NOISE

Figure S5 shows a normalized plot of the PL-detected and heterodyne-detected photon-echo decay profiles of Figs. 3(c) and 3(d) of the main text in comparison with the two measurements' relative noise floors. The raw values of these two noise floors are different from each other because of the inherent differences of the two different signal collection schemes. To facilitate a more direct comparison, the plots have been normalized to the values of best-fit lines at time $t = 0$. As shown by the graph, the slight deviation between the data and mono-exponential best fit line at times $t + \tau > 300$ ps is a result of the

measurement's noise floor and should not be attributed to an additional component in the decay curves relaxation dynamics. To the extent that an additional component of the PL-detected curve might exist, it must still be significantly smaller than its counterpart in the heterodyne-detected curve. In regions where the background noise does not impact the data (for example, at $t + \tau = 250$ ps) the normalized signal of the heterodyne-detected measurement remains significantly above that of the PL-detected measurement.

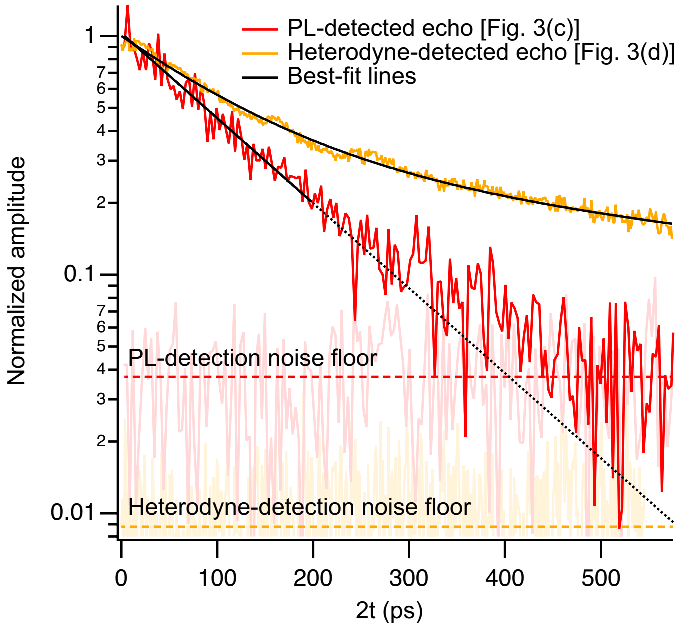


FIG. S5. Photon-echo relaxation plots from Figs. 3(c) and 3(d) of the main text, normalized to the values of their respective best-fit lines at time $t = 0$ ps. The noise floors correspond to an average of the background counts from horizontal line-outs of the data sets from Figs. 3(a) and 3(b) at $\tau = 250$ ps. The light pink trace is a line-out from Fig. 3(a) at $\tau = t + (75\text{ ps})$. The light orange trace is a line-out from Fig. 3(b) at $\tau = t + (15\text{ ps})$.

## EXTRACTION OF $T_1$ DECAY TIMES

Measurements of the $T_1$ population decay time were extracted for both PL-detected and heterodyne-detected MDCS experiments by varying the stage corresponding to the intermediate waiting time $T$ in Figs. S3 and S4 while holding the delay stages controlling the $\tau$ and $t$ delay times fixed and at delay values equal to each other. For the PL-detected measurement, we observed the signal to decay smoothly with $T$, exhibiting an appreciable

signal amplitude of at even the full extent of the delay stage's 935-ps scanning range. The same was true of the heterodyne measurement, although in this case the measurement turned out to be more strongly affected by angular variations of the delay stage mirrors, resulting in an increased amount of systematic error. In all cases the $T_1$ time appears to be on the order of 1–2 ns, which is consistent with other measurements in the $SiV^-$ literature.

## AUXILIARY MEASUREMENTS

To verify that the heterodyne-detected measurements reported in the main text correspond to an inhomogeneous population of $SiV^-$ hidden states and not a measurement artifact or signature of another type of color center, we performed a systematic excitation-frequency dependence of the heterodyne-detected measurement, as shown in Fig. S6, and we performed a series of conventional absorption measurements on the sample, as shown in Fig. S7. To our knowledge, the only other relevant defect-based spectral signature in the frequency range of our measurements is the GR1 line at 404.5 THz (1.673 eV), i.e., the zero-phonon line of the neutrally charged carbon vacancy [9]. As shown by Fig. S6, however, the maximal brightness of the hidden-center resonance when the laser center frequency is tuned near 404.5 THz is less than 30% of the maximal brightness when it is tuned near the 406.8 THz (1.682 eV) resonance associated with $SiV^-$ centers [compare Figs. S6(b) and S6(d)]. When the laser center frequency is tuned halfway between the two resonance lines [Fig. S6(c)], the spectral intensity is skewed decidedly toward the $SiV^-$ center lines. The absorption measurement of Fig. S7, which is not a bandwidth-impacted measurement, exhibits similar characteristics and moreover confirms that the inhomogeneous hidden-center population can be detected using linear spectroscopy methods in addition to MDCS.

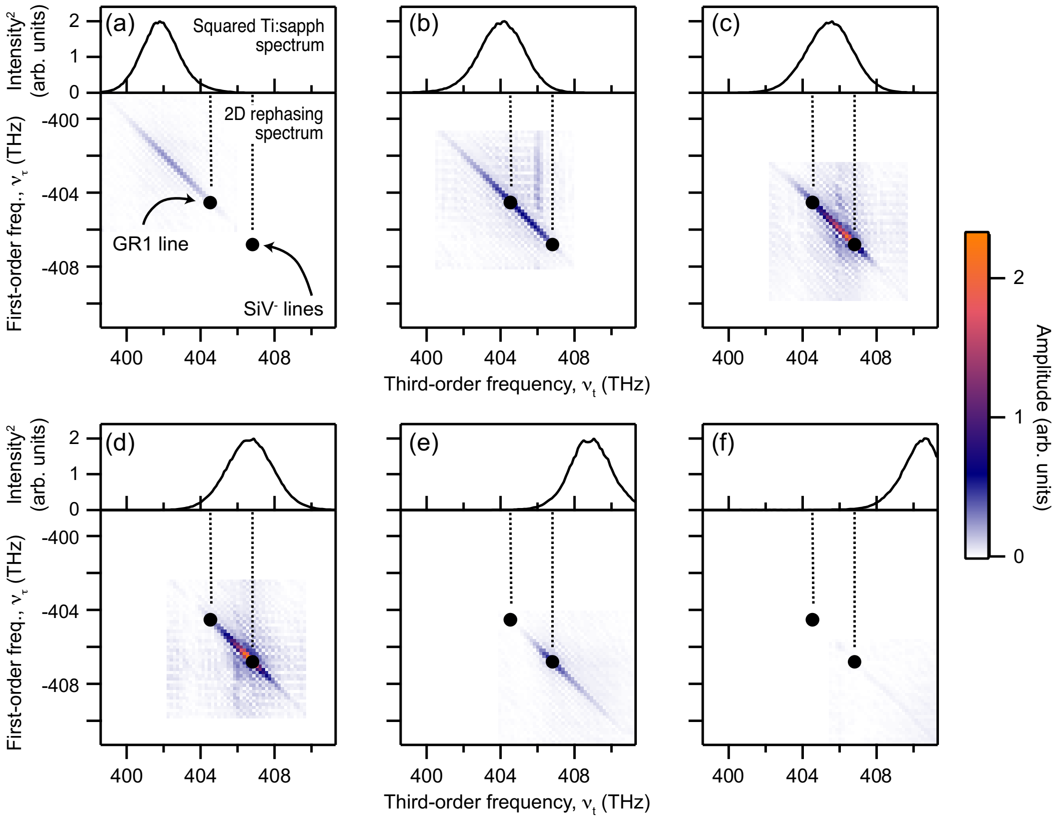


FIG. S6. A series of MDCS spectra taken with different excitation laser center frequencies. The top panels are measured squared laser spectra. The bottom panels are the associated 2D rephasing spectra.

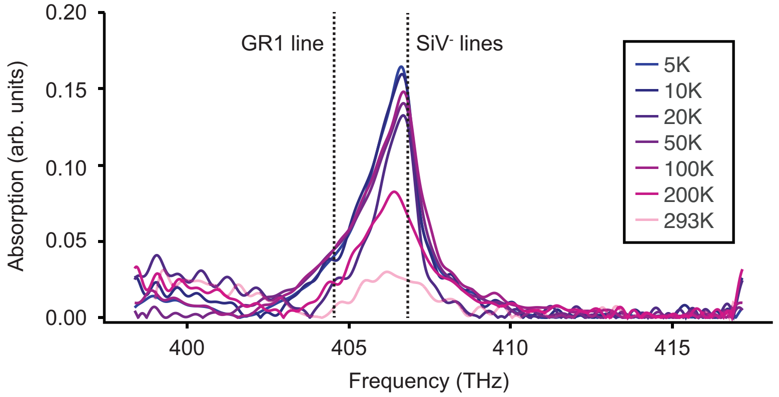


FIG. S7. Temperature-dependent linear absorption measurements of the $SiV^-$ center sample.

## THEORETICAL MODEL

To illustrate our interpretation of MDCS results, we present in this section a simplified model of the filtering effect that photoluminescence detection can impose in a system with nonradiative decay channels. We consider a system in which a common external forcing function like strain exerts a dual effect on an open two-level system, shifting the system's optically resonant frequencies while simultaneously enhancing the coupling effects between the bright state $|1\rangle$ and a nearby dark state $|2\rangle$ for which emission cannot be observed. (The existence and relevance of such a dark state is supported by Refs. [10–12].) An energy-level diagram corresponding to the system is displayed in Fig. S8(a), and two possible scenarios—discussed in more detail below—under which this coupling enhancement might occur are depicted by the graphs in Figs. S8(b) and S8(c).

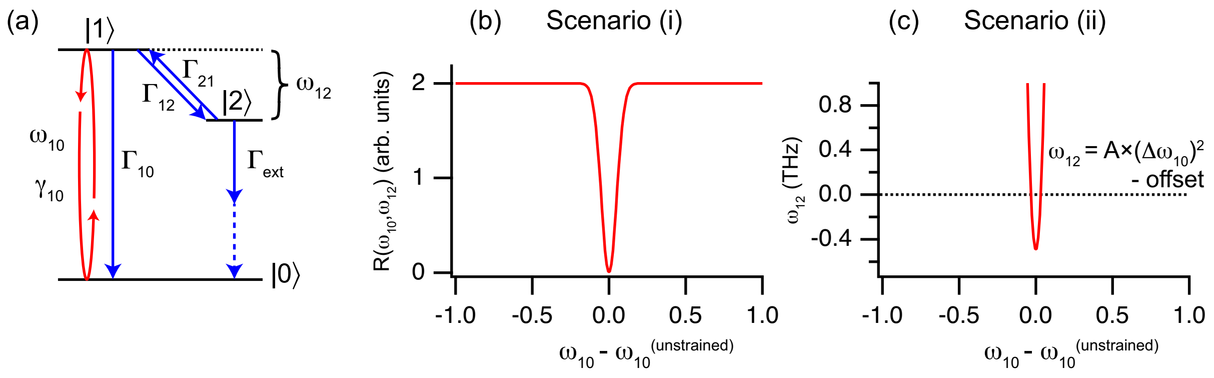


FIG. S8. Theoretical model parameters and inputs. **(a)** Energy level diagram. **(b)** Scenario in which $\omega_{10}$ is correlated with the electron-phonon coupling parameter $R$. **(c)** Scenario in which $\omega_{10}$ is correlated with the frequency separation $\omega_{12}$.

The dynamics of this system's density matrix can be modeled using the rate equations

$$\dot{\rho}_{10} = -(i\omega_{10} + \gamma_{10})\rho_{10} + \frac{i}{\hbar} V_{10} (\rho_{11} - \rho_{00}) \tag{s1}$$

$$\dot{\rho}_{11} = -\Gamma_{10}\rho_{11} - \Gamma_{12}\rho_{11} + \Gamma_{21}\rho_{22} - \frac{i}{\hbar} (V_{10}\rho_{01} - \rho_{10}V_{01}) \tag{s2}$$

$$\dot{\rho}_{22} = -\Gamma_{ext}\rho_{22} + \Gamma_{12}\rho_{11} - \Gamma_{21}\rho_{22} \tag{s3}$$

$$\dot{\rho}_{00} = \Gamma_{10}\rho_{11} + \Gamma_{ext}\rho_{22} + \frac{i}{\hbar} (V_{10}\rho_{01} - \rho_{10}V_{01}) \tag{s4}$$

with $\Gamma_{12}$ and $\Gamma_{21}$ being frequency-dependent functions,

$$\Gamma_{12}(\omega_{10},\omega_{12}) = R(\omega_{10},\omega_{12})\,[n(\omega_{12})+1]\,\mathrm{sgn}(\omega_{12}) \tag{s5}$$

$$\Gamma_{21}(\omega_{10},\omega_{12}) = R(\omega_{10},\omega_{12}) n(\omega_{12}) \mathrm{sgn}(\omega_{12}). \tag{s6}$$

The parameters $V_{10}$ and $V_{01}$ are interaction Hamiltonian matrix elements. The rate $\Gamma_{10}$ is the radiative decay rate from state $|1\rangle$ back into the ground state, and $\Gamma_{12}$, $\Gamma_{21}$, and $\Gamma_{ext}$ are nonradiative decay rates associated with state $|2\rangle$ as indicated in Fig. S8(a). The parameter $R(\omega_{10},\omega_{12})$ is an electron-phonon coupling function, and $n(\omega_{12}) \equiv 1/[e^{\beta\hbar\omega_{12}}-1]$ is the Bose-Einstein distribution function for a phonon bath at finite temperature. In addition to these effects, the system is modeled in the incoherent limit, which is to say that we assume that the relaxation timescales $T_1$ and $T_2$ are related according to $T_2 \ll 2T_1$, or alternatively, that

$$\gamma_{10} = \frac{1}{2}\left(\Gamma_{10}+\Gamma_{12}\right) + \gamma_c \quad \text{with} \quad \gamma_c \gg \frac{1}{2}\left(\Gamma_{10}+\Gamma_{12}\right), \tag{s7}$$

where $(\Gamma_{10}+\Gamma_{12}) \geq 1/T_1$, $\gamma_{10} = 1/T_2$, and $\gamma_c$ is the collisional or "pure" dephasing rate for processes in which the mutual coherence of states $|0\rangle$ and $|1\rangle$ is lost without any corresponding change in population [13].

Taking the above parameters as given, the associated MDCS measurements under heterodyne-detection and PL-detection scenarios can be calculated using density matrix perturbation theory [14] under circumstances where the interacting electromagnetic excitation pulses are treated as being of infinitesimally short duration. The waiting time $T$ between the second and third of these pulses is assumed to be short, such that $0 < T \ll T_1$.

**Heterodyne detection:**

For the heterodyne-detected measurement, the spectroscopic signal emerges from the product of the dipole matrix element $\mu = \langle 1|e\hat{r}|0\rangle$ with the phase-matched component of the third-order density matrix correction $\rho^{(3)}_{10}$, given in the time domain by

$$I_{sig}(t,\tau) \propto \; \mathrm{Re}\left\{\int_{-\infty}^{\infty} \tilde{E}^{*}_{LO}(s-t)\left[i\,\mu^{*}\rho^{(3)}_{10,sig}(s,\tau)\right] ds\right\}, \text{ with} \tag{s8}$$

$$\rho^{(3)}_{10,sig}(t,\tau) = -\frac{i|\mu|^2\mu}{8\hbar^3}\Theta(t)e^{-i[\omega_{10}-i\gamma_{10}]t}\Theta(\tau)e^{-i[-\omega_{10}-i\gamma_{10}]\tau} \tag{s9}$$

and in the frequency domain by

$$I_{sig}(\omega_t, \omega_\tau) \propto \tilde{E}^*_{LO}(-\omega_t) \left[ i\mu^* \rho^{(3)}_{10,sig}(\omega_t, \omega_\tau) \right], \text{ with} \tag{s10}$$

$$\rho^{(3)}_{10,sig}(\omega_t, \omega_\tau) = -\frac{i|\mu|^2\mu}{8\hbar^3} \left( \frac{i}{\omega_t - [\omega_{10} - i\gamma_{10}]} \right) \left( \frac{i}{\omega_\tau - [-\omega_{10} - i\gamma_{10}]} \right). \tag{s11}$$

Because the timescale of emission is on the order of $T_2 \ll T_1$, there are no measurable effects under these circumstances of the influence of the dark state.

**Photoluminescence detection:**

For the PL-detected measurement, the spectroscopic signal emerges from the phase-matched component of the fourth-order density matrix correction $\rho^{(4)}_{11}$, given in the time domain by

$$I_{sig}(t, \tau) \propto B(\omega_{10}, \omega_{12}) \text{ Re} \left\{ \rho^{(4)}_{11,sig}(t, \tau) \right\}, \text{ with} \tag{s12}$$

$$\rho^{(4)}_{11,sig}(t, \tau) = \frac{|\mu|^4}{16\hbar^4} \Theta(t) e^{-i[\omega_{10} - i\gamma_{10}]t} \Theta(\tau) e^{-i[-\omega_{10} - i\gamma_{10}]\tau} \tag{s13}$$

and in the frequency domain by

$$I_{sig}(\omega_t, \omega_\tau) \propto B(\omega_{10}, \omega_{12}) \ \rho^{(4)}_{11,sig}(\omega_t, \omega_\tau), \text{ with} \tag{s14}$$

$$\rho^{(4)}_{11,sig}(\omega_t, \omega_\tau) = \frac{|\mu|^4}{16\hbar^4} \left( \frac{i}{\omega_t - [\omega_{10} - i\gamma_{10}]} \right) \left( \frac{i}{\omega_\tau - [-\omega_{10} - i\gamma_{10}]} \right) \tag{s15}$$

Importantly, however, this signal is only observed to the extent that the population decays by radiative emission, and so signal filtering can occur in response to different types of physical mechanisms through the parameter $B(\omega_{10}, \omega_{12})$, as we now proceed to outline under two separate scenarios.

*Scenario (i):* Perhaps the most straightforward filtering mechanism is the case where the electron-phonon coupling function $R(\omega_{10}, \omega_{12})$ is suppressed in the absence of strain and enhanced in its presence as depicted in Fig. S8(b). Such a correlation would be expected to occur if, for example, the transition between states $|1\rangle$ and $|2\rangle$ is forbidden by symmetry in the unstrained system. Because the application of strain is a symmetry-breaking process, this transition pathway would be expected to open up as the resonant frequency $\omega_{10}$ shifts increasingly away from $\omega_{10}^{(\text{unstrained})}$. To keep the illustration simple, we set $\Gamma_{10}$ to a constant and let the frequency $\omega_{12}$ be large enough to suppress feedback effects resulting

from the population of $\rho_{22}$ flowing back into $\rho_{11}$. The overall effect is that the PL-detected measurement will be filtered by the branching ratio

$$B(\omega_{10}, \omega_{12}) = \frac{\Gamma_{10}}{\Gamma_{10} + \Gamma_{12}(\omega_{10}, \omega_{12})} \approx \frac{\Gamma_{10}}{\Gamma_{10} + R(\omega_{10}, \omega_{12})}. \tag{s16}$$

*Scenario (ii):* An alternate filtering mechanism is a circumstance in which strain shifts the system's energy levels in such a manner that $\omega_{12}$ shifts in the same direction for both positive and negative values of $\omega_{10} - \omega_{10}^{(\text{unstrained})}$ as depicted in Fig. S8(c). If the unstrained energy of state $|2\rangle$ lies above that of state $|1\rangle$ and if the effect of strain is sufficient to drive this energy to below that of state $|1\rangle$, then the decay rate $\Gamma_{12}$ will be enhanced by the ability of state $|1\rangle$ to decay into state $|2\rangle$ through spontaneous phonon emission as the transition frequency $\omega_{12}$ goes from negative to positive. The results of this scenario can be readily approximated in two limits. In the limit of $\Gamma_{ext} \gg \Gamma_{21}$, then the population term $\rho_{22}$ will remain small at all times and the PL-detected signal will be suppressed by the branching ratio

$$B(\omega_{10}, \omega_{12}) = \frac{\Gamma_{10}}{\Gamma_{10} + \Gamma_{12}(\omega_{10}, \omega_{12})}. \tag{s17}$$

Although this may look almost the same as the branching ratio of Eq. (s16), there is an important difference between the two functions in that the Bose-Einstein distribution function's presence in Eq. (s5) can be ignored in the formulation of Eq. (s16) but not in the formulation of Eq. (s17). In the opposing limit of $\Gamma_{10} \ll \Gamma_{21}$ and $\Gamma_{ext} \ll \Gamma_{21}$, then states $|1\rangle$ and $|2\rangle$ establish a quasi-thermal equilibrium before decaying back to the ground state. As a condition of this equilibrium, the occupancies of states $|1\rangle$ and $|2\rangle$ will be related to each other by the Boltzmann factor $\rho_{11}/\rho_{22} = e^{-\beta\hbar\omega_{12}}$, leading to a PL-detected signal that will be subject to the filter function

$$B(\omega_{10}, \omega_{12}) = \frac{\Gamma_{10}}{\Gamma_{10} + \Gamma_{ext} e^{\beta\hbar\omega_{12}}}. \tag{s18}$$

**Simulation results:**

Having established these relations, we proceed to examine a more comprehensive ensemble of $N$ two-level systems in which inhomogeneous strain induces a correspondingly inhomogeneous set of resonance frequencies $\{\omega_{10}\}$, which we model as being distributed about the unstrained resonant frequency $\omega_{10}^{(\text{unstrained})}$ with inhomogeneity parameter $\sigma$ as specified by

the Gaussian function

$$G\left(\omega_{10}-\omega_{10}^{(\text{unstrained})}\right) \equiv \frac{N}{\sigma\sqrt{2\pi}} \exp\left[\frac{-\left(\omega_{10}-\omega_{10}^{(\text{unstrained})}\right)^2}{2\sigma^2}\right]. \tag{s19}$$

The resulting MDCS signals can be computed as a weighted sum of the one-particle signals, expressible in integral form by generalizing the terms inside Eqs. (s10) and (s14) to be explicit functions of $\omega_{10}$ and cross-correlating with the distribution function to obtain

$$I_{tot,het}(\omega_t,\omega_\tau) \propto \tilde{E}^*_{LO}(-\omega_t) \int_{-\infty}^{\infty} G\left(\omega_{10}-\omega_{10}^{(\text{unstrained})}\right) \left[i\mu^* \rho^{(3)}_{10,sig}(\omega_t,\omega_\tau,\omega_{10})\right] d\omega_{10} \tag{s20}$$

and

$$I_{tot,PL}(\omega_t,\omega_\tau) \propto \int_{-\infty}^{\infty} G\left(\omega_{10}-\omega_{10}^{(\text{unstrained})}\right) B(\omega_{10},\omega_{12})\ \rho^{(4)}_{11,sig}(\omega_t,\omega_\tau,\omega_{10})\, d\omega_{10}. \tag{s21}$$

Numerically computed MDCS spectra corresponding to this integral in the heterodyne-detection case and in the PL-detection case under Scenario (i) are shown in Fig. S9 and reproduced in Fig. 4 of the main text. Spectra corresponding to PL-detection under Scenario (ii) in the two opposing limits of $\Gamma_{ext} \gg \Gamma_{21}$ and $\Gamma_{ext}$, $\Gamma_{10} \ll \Gamma_{21}$ are shown in Fig. S10.

As shown in Figs. S9(a) and S9(b), the heterodyne-detected MDCS spectrum is completely independent of branching-ratio filtering effects and as such exhibits a diagonal linewidth that is dominated by the parameter $\sigma$. By contrast, the PL-detected spectrum is correlation-function-dependent. Figures S9(c)–S9(e) and their associated projections in Figs. S9(f)–S9(h) show the results of PL-detected MDCS simulations under Scenario (i) as described in the previous section under circumstances where the electron-phonon coupling function $R(\omega_{10},\omega_{12})$ is as depicted in Fig. S8(b) under circumstances where the limit of $R(\omega_{10},\omega_{12})/\Gamma_{10}$ as $\omega_{10}-\omega_{10}^{(\text{unstrained})} \to \infty$ is respectively given by 0.1, 1, and 10. While the filtering effect exerts an only minor influence on the data when $R/\Gamma_{10} \to 0.1$, it becomes a significant factor when $R/\Gamma_{10} \to 1$ and is the dominant source of the diagonal linewidth for values of $R/\Gamma_{10} \to 10$ or larger.

Figure S10 shows the results of PL-detected MDCS simulations under Scenario (ii) as described in the previous section under circumstances where the nonradiative decay frequency $\omega_{12}$ depends on the radiative decay frequency $\omega_{10}$ according to the function in Fig. S8(c). The electron-phonon coupling function $R(\omega_{10},\omega_{12})$ has little-to-no strain dependence directly, but is rather simulated according to the Debye model as a quadratic

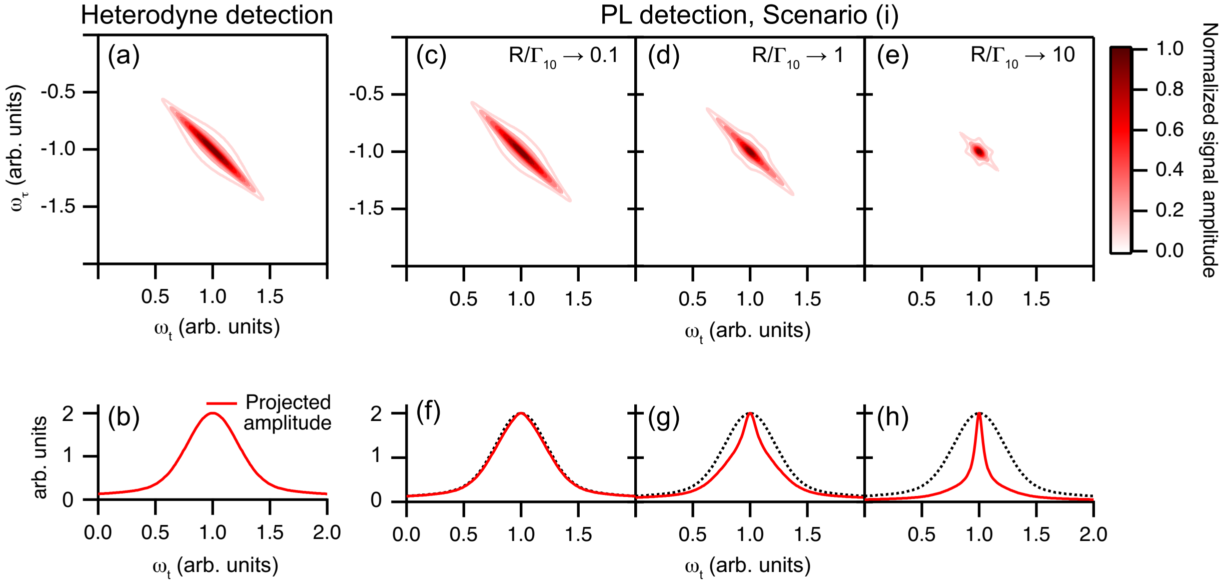


FIG. S9. Heterodyne detection vs. PL detection simulation results. **(a)** Simulated heterodyne-detected MDCS plot resulting from Eq. (s20) under circumstances of $\sigma = 0.2\,\omega_{10}^{(\text{unstrained})}$, where $\gamma_{10} = 0.05\,\sigma$ is assumed to be dominated by $\gamma_c$. **(b)** Projection from (a) onto the $\omega_t$ axis. **(c)–(e)** Simulated PL-detected MDCS plots resulting from Eq. (s21) under circumstances of $R/\Gamma_{10} \to 0.1$, 1, and 10, respectively. **(f)–(h)** Projection onto the $\omega_t$ axis of the amplitude plots depicted in (a)–(d). The dotted black lines in panels (f)–(h) are duplicates of the solid red line depicted in panel (b).

function $R(\omega_{10}, \omega_{12}) = R(\omega_{12}) \propto \omega_{12}^2$. Figures S10(a)–S10(f) show simulation results of this model in the limit $\Gamma_{ext} \gg \Gamma_{21}$, where the multiplication parameter $A = 5 \times 10^{12}$ THz$/\omega_{10}^2$, $50 \times 10^{12}$ THz$/\omega_{10}^2$, and $500 \times 10^{12}$ THz$/\omega_{10}^2$, and where the temperature is 10 K. Figures S10(g)–S10(l) show simulation results of this model in the limit where $\Gamma_{ext}, \Gamma_{10} \ll \Gamma_{21}$ under the same three values of $A$. In both cases it is possible to increase the mutliplication factor to the point where filtering effects are the dominant contribution to the observed inhomogeneity in the photoluminescence-detected spectrum.

We note in closing that the model as we have presently constructed does not reproduce the experimental fact that the heterodyne measurement exhibits $T_2$ times that exceed the $T_2$ times of the PL-detected measurement. Such effects can be captured, however, by adding an additional correlation between strain and the parameter $\gamma_c$.

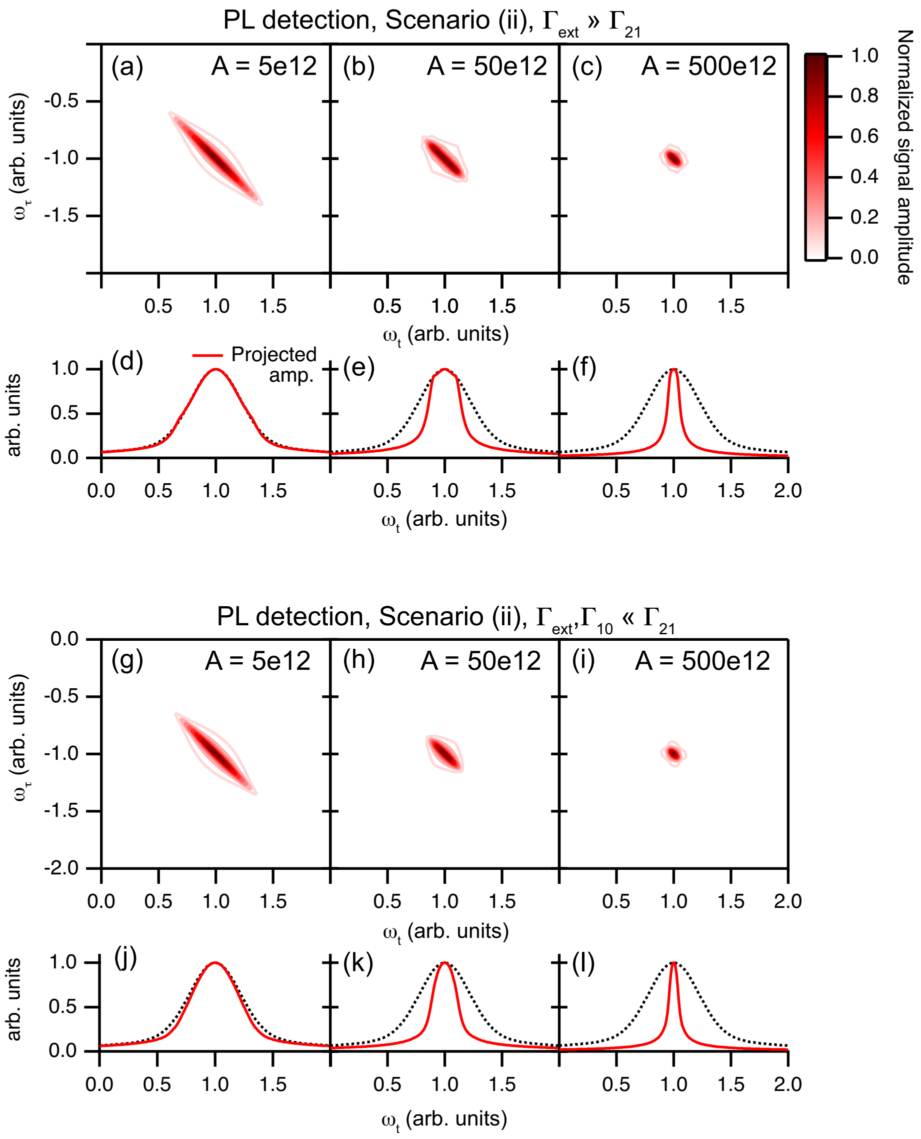


FIG. S10. PL detection simulation results under Scenario (ii). **(a)–(f)** Simulated PL-detected MDCS plots and associated amplitude projections under circumstances where $\Gamma_{ext} \gg \Gamma_{21}$, for three different values of the multiplication parameter $A$ as defined in Fig. S8(c). **(g)–(l)** Simulated PL-detected MDCS plots and associated amplitude projections under the same values of $A$ under circumstances where $\Gamma_{ext}$, $\Gamma_{10} \ll \Gamma_{21}$.

---

* Present address: HRL, Malibu, CA 90265 USA

† Present address: Department of Physics, University of Washington, Seattle, WA 98195, USA

‡ Email: cundiff@umich.edu

[1] S. Lindner, A. Bommer, A. Muzha, A. Krueger, L. Gines, S. Mandal, O. Williams, E. Londero, A. Gali, and C. Becher, New J. Phys. **20**, 115002 (2018).

[2] S. Meesala, Y.-I. Sohn, B. Pingault, L. Shao, H. A. Atikian, J. Holzgrafe, M. Gündoğan, C. Stavrakas, A. Sipahigil, C. Chia, R. Evans, M. J. Burek, M. Zhang, L. Wu, J. L. Pacheco, J. Abraham, E. Bielejec, M. D. Lukin, M. Atatüre, and M. Lončar, Phys. Rev. B **97**, 205444 (2018).

[3] M. V. Hauf, B. Grotz, B. Naydenov, M. Dankerl, S. Pezzagna, J. Meijer, F. Jelezko, J. Wrachtrup, M. Stutzmann, F. Reinhard, and J. A. Garrido, Phys. Rev. B **83**, 081304 (2011).

[4] C. Osterkamp, J. Lang, J. Scharpf, C. Müller, L. P. McGuinness, T. Diemant, R. J. Behm, B. Naydenov, and F. Jelezko, Appl. Phys. Lett. **106**, 113109 (2015).

[5] T. Schröder, M. E. Trusheim, M. Walsh, L. Li, J. Zheng, M. Schukraft, A. Sipahigil, R. E. Evans, D. D. Sukachev, C. T. Nguyen, J. L. Pacheco, R. M. Camacho, E. S. Bielejec, M. D. Lukin, and D. Englund, Nat. Commun. **8**, 15376 (2017).

[6] P. F. Tekavec, G. A. Lott, and A. H. Marcus, J. Chem. Phys. **127**, 214307 (2007).

[7] G. Nardin, T. M. Autry, K. L. Silverman, and S. T. Cundiff, Opt. Express **21**, 28617 (2013).

[8] E. W. Martin and S. T. Cundiff, Phys. Rev. B **97**, 081301 (2018).

[9] G. Davies and C. Foy, J. Phys. C: Solid State Phys. **13**, 2203 (1980).

[10] E. Neu, M. Agio, and C. Becher, Opt. Express **20**, 19956 (2012).

[11] E. Neu, R. Albrecht, M. Fischer, S. Gsell, M. Schreck, and C. Becher, Phys. Rev. B **85**, 245207 (2012).

[12] A. Gali and J. R. Maze, Phys. Rev. B **88**, 235205 (2013).

[13] R. W. Boyd, *Nonlinear Optics*, 3rd ed. (Elsevier, Waltham, MA, 2009) p. 283.

[14] P. Hamm and M. Zanni, *Concepts and Methods of 2D Infrared Spectroscopy* (Cambridge University Press, 2011).
